# Supplementary material for: Optimizing Reported Age of Information with Short Error Correction and Detection Codes
Source: arXiv:2309.05974 source file (2023-09-12)
Supplement: Supplementary file 1 [file Appendix.tex]

\subsection{Proof of Theorem 2}\label{Thm:2-proof}
For proving Theorem \ref{threshold_struct}, we need the following lemma, where we show that the value function is non-decreasing in the age of user $m$ when other state variables are fixed.
\begin{lemma}
When $\mathbf{a}_{-m}$ and $\mathbf{h}$ are fixed, the value function $V_{\boldsymbol{\lambda},\gamma,n}(a_m,\mathbf{a}_{-m}, \mathbf{h})$ is a non-decreasing function of $a_m$. 
\end{lemma}
\begin{proof}
We prove the result via induction. Consider the following Bellman equation: 
	\begin{flalign}\label{eq:val_iter}
		& V_{n+1}(a_m,\cdot) &&\nonumber \\ 
		&\;\; = \min_{\mathbf{I}_{e},\mathbf{I}_{l}, \boldsymbol{\theta}} \left( c_{\boldsymbol{\lambda}}(a_m,I_{e},I_{l}, \boldsymbol{\theta},\cdot)+ \gamma \mathbb{E}[V_{n}(\mathbf{s}')|a_m,I_{e},I_{l}, \boldsymbol{\theta},\cdot]\right),&&
	\end{flalign}
	where $(\cdot)$ represents the fixed quantities and the next state, $\mathbf{s}'=(a_m',\mathbf{a}_{-m}',\mathbf{h}')$. The trade-off parameter, $\boldsymbol{\lambda} $ and the discount factor, $\gamma$ in $V_{\boldsymbol{\lambda},\gamma,n}$ are dropped for simplicity. Since $V_0(a_m,\cdot)\triangleq0$, $V_0(a_m,\cdot)$ is non-decreasing in $a_m$.  For completing the proof via induction, it is required to show that $V_{n+1}(a_m,\cdot)$ is non-decreasing in $a_m$  whenever $V_n(a_m,\cdot)$ is non-decreasing in $a_m$. 
    For this, note that the minimum operator preserves the non-decreasing behavior and the instantaneous cost, \eqref{cost} is non-decreasing in $a_m$. Hence, referring to  \eqref{eq:val_iter},   it only  remains to prove that  $\mathbb{E}[V_n(\mathbf{s}')|a_m, I_{e,m}, I_{l,m},\boldsymbol{\theta},\cdot]$ is non-decreasing in $a_m$, i.e.,  
    	\begin{align}\label{exptn_v}
    &\mathbb{E}[V_n(\mathbf{s}'|a_m+1, I_{e,m}, I_{l,m},\boldsymbol{\theta},\cdot)] \nonumber\\ 
    & \qquad \qquad \qquad \geq \mathbb{E}[V_n(\mathbf{s}'|a_m, I_{e,m}, I_{l,m},\boldsymbol{\theta},\cdot)],
    \end{align}
    holds true for different valid combinations of $I_{e,m}$ and $I_{l,m}$ and for any decoding order $\boldsymbol{\theta}$. 
    For proving \eqref{exptn_v}, we consider several cases in the below.   
    
	\textit{Case 1:}  When $I_{e,m}=0$ and $I_{l,m}=0$, for state $\mathbf{s} =(a_m,\mathbf{a}_{-m}, \mathbf{h})$, the next state, $\mathbf{s}'=(a_m+1,\mathbf{a}_{-m}',\mathbf{h}')$. Hence,
%	\begin{align*}
%		&\mathbb{E}[V_n(\mathbf{s}'_2)|a_m+1, I_{e,m}=0, I_{l,m}=0,\boldsymbol{\theta},\cdot] \\
%		= & \sum_{\mathbf{s}'_2 \in  \mathcal{M}} \mathbb{P}\left(\mathbf{s}'_2|a_m+1,I_{e,m}=0,I_{l,m}=0,\boldsymbol{\theta},\cdot\right)V_n(\mathbf{s}'_2)\\
%		 \stackrel{b}\geq & \sum_{\mathbf{s}'_1 \in  \mathcal{M}} \mathbb{P}(\mathbf{s}'_1|a_m,I_{e,m}=0,I_{l,m}=0,\boldsymbol{\theta},\cdot)V_n(\mathbf{s}'_1)\\  
%		 = & \; \mathbb{E}[V_n(\mathbf{s}'_1)|a_m, I_{e,m}=0, I_{l,m}=0,\boldsymbol{\theta},\cdot],
%	\end{align*}
$\mathbb{E}[V_n(\mathbf{s}'_2)|a_m+1, I_{e,m}=0, I_{l,m}=0,\boldsymbol{\theta},\cdot] =  \sum_{\mathbf{s}'_2 \in  \mathcal{M}} \mathbb{P}\left(\mathbf{s}'_2|a_m+1,I_{e,m}=0,I_{l,m}=0,\boldsymbol{\theta},\cdot\right)V_n(\mathbf{s}'_2)\stackrel{b}\geq \sum_{\mathbf{s}'_1 \in  \mathcal{M}} \mathbb{P}(\mathbf{s}'_1|a_m,I_{e,m}=0,I_{l,m}=0,\boldsymbol{\theta},\cdot)V_n(\mathbf{s}'_1)=  \mathbb{E}[V_n(\mathbf{s}'_1)|a_m, I_{e,m}=0, I_{l,m}=0,\boldsymbol{\theta},\cdot],$
where $\mathbf{s}'_1=(a_m+1,\mathbf{a}_{-m}',\mathbf{h}')$, $\mathbf{s}'_2=(a_m+2,\mathbf{a}_{-m}',\mathbf{h}')$. Here (b) holds true because of the assumption that $V_n(a_m,\cdot)$ is non-decreasing in $a_m$ and due to
\begin{equation}\label{prob_rho}
			\mathbb{P}(\mathbf{s}'= (a'_m,\mathbf{a}'_{-m}, \mathbf{h}')|a_m, I_{e,m}, I_{l,m},\boldsymbol{\theta},\cdot)= \mathbb{P}(\mathbf{h}'). 
	\end{equation} Therefore, \eqref{exptn_v} holds true for $I_{e,m}=0$ and $I_{l,m}=0$.
	
	\textit{Case 2:}  When $I_{e,m}=0$ and $I_{l,m}=1$, now for state, $\mathbf{s} =(a_m,\mathbf{a}_{-m}, \mathbf{h})$, the next state, $\mathbf{s}'=(1,\mathbf{a}_{-m}',\mathbf{h}')$. Hence,	 $ \mathbb{E}[V_n(\mathbf{s}')|a_m+1, I_{e,m}=0, I_{l,m}=1,\boldsymbol{\theta},\cdot] 
		= \sum_{\mathbf{s}' \in  \mathcal{M}} \mathbb{P}(\mathbf{s}'|a_m+1,I_{e,m}=0,I_{l,m}=1,\boldsymbol{\theta},\cdot)V_n(\mathbf{s}')
		\stackrel{c} =
		\sum_{\mathbf{s}' \in  \mathcal{M}} \mathbb{P}(\mathbf{s}'|a_m,I_{e,m}=0,I_{l,m}=1,\boldsymbol{\theta},\cdot)V_n(\mathbf{s}')  
		= \mathbb{E}[V_n(\mathbf{s}')|a_m, I_{e,m}=0, I_{l,m}=1,\boldsymbol{\theta},\cdot],$
%	\begin{align*}
%		&\mathbb{E}[V_n(\mathbf{s}')|a_m+1, I_{e,m}=0, I_{l,m}=1,\boldsymbol{\theta},\cdot] \\ 
%		= & \sum_{\mathbf{s}' \in  \mathcal{M}} \mathbb{P}(\mathbf{s}'|a_m+1,I_{e,m}=0,I_{l,m}=1,\boldsymbol{\theta},\cdot)V_n(\mathbf{s}')\\
%		\stackrel{c} = &
%		\sum_{\mathbf{s}' \in  \mathcal{M}} \mathbb{P}(\mathbf{s}'|a_m,I_{e,m}=0,I_{l,m}=1,\boldsymbol{\theta},\cdot)V_n(\mathbf{s}')\\  
%		= & \mathbb{E}[V_n(\mathbf{s}')|a_m, I_{e,m}=0, I_{l,m}=1,\boldsymbol{\theta},\cdot],
%	\end{align*}
	where (c) holds true with equality due to \eqref{prob_rho}
and whether $\mathbf{s} = (a_m,\mathbf{a}_{-m}, \mathbf{h})$ or $\mathbf{s}=(a_m+1,\mathbf{a}_{-m}, \mathbf{h})$, the next state, $\mathbf{s}'=(1,\mathbf{a}_{-m}',\mathbf{h}')$. Therefore, \eqref{exptn_v}   holds true when $I_{e,m}=0$ and $I_{l,m}=1$.
	
	\textit{Case 3}:  When $I_{e,m}=1$ and $I_{l,m}=0$, irrespective of whether present state $\mathbf{s} =(a_m,\mathbf{a}_{-m}, \mathbf{h}) $ or $\mathbf{s} =(a_m+1,\mathbf{a}_{-m}, \mathbf{h}) $, the next state $\mathbf{s}'=(1,\mathbf{a}_{-m}',\mathbf{h}')$. Hence, $\mathbb{E}[V_n(\mathbf{s}'|a_m+1, I_{e,m}=1, I_{l,m}=0,\boldsymbol{\theta},\cdot)] = \sum_{\mathbf{s}' \in  \mathcal{M}} \mathbb{P}(\mathbf{s}'|a_m+1,I_{e,m}=1,I_{l,m}=0,\boldsymbol{\theta},\cdot)V_n(\mathbf{s}')
		\stackrel{d}= 
		\sum_{\mathbf{\mathbf{s}}' \in  \mathcal{M}} \mathbb{P}(\mathbf{s}'|a_m,I_{e,m}=1,I_{l,m}=0,\boldsymbol{\theta},\cdot)V_n(\mathbf{s}')
		= \mathbb{E}[V_n(\mathbf{s}'|a_m, I_{e,m}=1, I_{l,m}=0,\boldsymbol{\theta},\cdot)],$
%	\begin{align*}
%		&\mathbb{E}[V_n(\mathbf{s}'|a_m+1, I_{e,m}=1, I_{l,m}=0,\boldsymbol{\theta},\cdot)] \\ = & \sum_{\mathbf{s}' \in  \mathcal{M}} \mathbb{P}(\mathbf{s}'|a_m+1,I_{e,m}=1,I_{l,m}=0,\boldsymbol{\theta},\cdot)V_n(\mathbf{s}')\\
%		\stackrel{d}= & 
%		\sum_{\mathbf{\mathbf{s}}' \in  \mathcal{M}} \mathbb{P}(\mathbf{s}'|a_m,I_{e,m}=1,I_{l,m}=0,\boldsymbol{\theta},\cdot)V_n(\mathbf{s}')\\ 
%		= & \mathbb{E}[V_n(\mathbf{s}'|a_m, I_{e,m}=1, I_{l,m}=0,\boldsymbol{\theta},\cdot)], 
%	\end{align*}
	where (d) holds true due to \eqref{prob_rho}. Therefore, \eqref{exptn_v}   holds true with equality for $I_{e,m}=1$ and $I_{l,m}=0$.
	
	\textit{Case 4:}  When $I_{e,m}=1$ and $I_{l,m}=1$, for state, $\mathbf{s} =(a_m,\mathbf{a}_{-m}, \mathbf{h})$, the next state will be, $\mathbf{s}'=(1,\mathbf{a}_{-m}',\mathbf{h}')$. Hence, $\mathbb{E}[V_n(\mathbf{s}')|a_m+1, I_{e,m}=1, I_{l,m}=1,\boldsymbol{\theta},\cdot]
		= \sum_{\mathbf{s}' \in  \mathcal{M}} \mathbb{P}\left(\mathbf{s}'|a_m+1,I_{e,m}=1,I_{l,m}=1,\boldsymbol{\theta},\cdot\right)V_n(\mathbf{s}')
		\stackrel{e}= 
		\sum_{\mathbf{s}' \in  \mathcal{M}} \mathbb{P}(\mathbf{s}'|a_m,I_{e,m}=1,I_{l,m}=1,\boldsymbol{\theta},\cdot)V_n(\mathbf{s}')  
		= \mathbb{E}[V_n(\mathbf{s}')|a_m, I_{e,m}=1, I_{l,m}=1,\boldsymbol{\theta},\cdot],$
%	\begin{align*}
%		&\mathbb{E}[V_n(\mathbf{s}')|a_m+1, I_{e,m}=1, I_{l,m}=1,\boldsymbol{\theta},\cdot] \\
%		 = & \sum_{\mathbf{s}' \in  \mathcal{M}} \mathbb{P}\left(\mathbf{s}'|a_m+1,I_{e,m}=1,I_{l,m}=1,\boldsymbol{\theta},\cdot\right)V_n(\mathbf{s}')\\ 
%		\stackrel{e}= & 
%		\sum_{\mathbf{s}' \in  \mathcal{M}} \mathbb{P}(\mathbf{s}'|a_m,I_{e,m}=1,I_{l,m}=1,\boldsymbol{\theta},\cdot)V_n(\mathbf{s}')\\  
%		= & \mathbb{E}[V_n(\mathbf{s}')|a_m, I_{e,m}=1, I_{l,m}=1,\boldsymbol{\theta},\cdot],
%	\end{align*}
	where (e) is true due to \eqref{prob_rho} and \eqref{exptn_v} holds with equality for $I_{e,m}=1$ and $I_{l,m}=1$.
  Hence,  $\mathbb{E}[V_n(\mathbf{s}'=a_m',\mathbf{a}_{-m}',$ $\mathbf{h}')|a_m, I_{e,m}, I_{l,m},\boldsymbol{\theta},\cdot]$ is a non-decreasing function in $a_m$.  
\end{proof}	

Using the above lemma, we prove Theorem 2 in the below. 
	\begin{proof}
 To prove that $I_{e,m}$ is non-decreasing in $a_m$ (and $h_m$) when other state-action variables are fixed, we consider two cases based on the two different values that $I_{l,m}$ can take and prove the result for each case separately.
	
    \textit{Case 1:}  When $I_{l,m}=0$,
	to show  $I_{e,m}$ is non-decreasing in $a_m$, it is sufficient to prove  $Q(a_m,\mathbf{a}_{-m}, \mathbf{h}, I_{e,m}, I_{l,m}=0, \mathbf{I}_{e,-m}, \mathbf{I}_{l,-m}, \boldsymbol{\theta})$ is sub-modular in $(a_m,I_{e,m})$, when $\mathbf{a}_{-m}, \mathbf{h}, \mathbf{I}_{e,-m}, \mathbf{I}_{l,-m} $ are fixed. %The fixed quantities are represented by $(.)$ in the below proof. 
	Consider
	\begin{align}
		&Q(a_m+1, I_{e,m}=1, I_{l,m}=0,\boldsymbol{\theta},\cdot) \nonumber  \\
		& \qquad \qquad \qquad \qquad -  Q(a_m+1, I_{e,m}=0, I_{l,m}=0,\boldsymbol{\theta},\cdot) \nonumber  \\
		&= w_m +\lambda_mP_{e,m}(h_m) \nonumber \\ &+\gamma\mathbb{E}\left[V(1,\mathbf{a}_{-m}',\mathbf{h}')|a_m+1, I_{e,m}=1, I_{l,m}=0,\boldsymbol{\theta},\cdot \right] \nonumber \\ 
		&- w_m ( a_m+2 ) \nonumber \\
		&-\gamma \mathbb{E}\left[V(a_m+2,\mathbf{a}_{-m}',\mathbf{h}')|a_m+1, I_{e,m}=0, I_{l,m}=0,\boldsymbol{\theta},\cdot\right]\nonumber\\
		&\stackrel{b}{\leq} w_m +  \lambda_mP_{e,m}(h_m) \nonumber  \\
		&+\gamma\mathbb{E}\left[V(1,\mathbf{a}_{-m}',\mathbf{h}')|a_m, I_{e,m}=1, I_{l,m}=0,\boldsymbol{\theta},\cdot \right] \nonumber \\ 
		&-w_m ( a_m+1) \nonumber  \\
		&-\gamma \mathbb{E}\left[V(a_m+1,\mathbf{a}_{-m}',\mathbf{h}')|a_m, I_{e,m}=0, I_{l,m}=0,\boldsymbol{\theta},\cdot\right] \nonumber  \\
		%1+\gamma\mathbb{E}\left[V(1)\right] - \left( a+1 +\gamma \mathbb{E}\left[V(s')|a, I_e=0, I_l=0\right]\right)\\
		&= Q(a_m, I_{e,m}=1, I_{l,m}=0,\boldsymbol{\theta},\cdot) \nonumber  \\
		& \qquad \qquad \qquad \qquad -  Q(a_m, I_{e,m}=0, I_{l,m}=0,\boldsymbol{\theta},\cdot),
	\end{align}
	where (b) holds true because, $\mathbb{E}[V(\mathbf{s}'_2)|a_m+1, I_{e,m}=0, I_{l,m}=0,\boldsymbol{\theta},\cdot]
	= \sum_{\mathbf{s}'_2 \in  \mathcal{M}} \mathbb{P}\left(\mathbf{s}'_2|a_m+1,I_{e,m}=0,I_{l,m}=0,\boldsymbol{\theta},\cdot\right)V(\mathbf{s}'_2) \stackrel{b'}\geq
	\sum_{\mathbf{s}'_1 \in  \mathcal{M}} \mathbb{P}(\mathbf{s}'_1|a_m,I_{e,m}=0,I_{l,m}=0,\boldsymbol{\theta},\cdot)V(\mathbf{s}'_1)=\mathbb{E}[V(\mathbf{s}'_1)|a_m, I_{e,m}=0, I_{l,m}=0,\boldsymbol{\theta},\cdot],$
%	\begin{align*}
%		& \mathbb{E}[V(\mathbf{s}'_2)|a_m+1, I_{e,m}=0, I_{l,m}=0,\boldsymbol{\theta},\cdot] \\
%		&= \sum_{\mathbf{s}'_2 \in  \mathcal{M}} \mathbb{P}\left(\mathbf{s}'_2|a_m+1,I_{e,m}=0,I_{l,m}=0,\boldsymbol{\theta},\cdot\right)V(\mathbf{s}'_2)\\ 
%		& \stackrel{b'}\geq
%		\sum_{\mathbf{s}'_1 \in  \mathcal{M}} \mathbb{P}(\mathbf{s}'_1|a_m,I_{e,m}=0,I_{l,m}=0,\boldsymbol{\theta},\cdot)V(\mathbf{s}'_1)\\  &=\mathbb{E}[V(\mathbf{s}'_1)|a_m, I_{e,m}=0, I_{l,m}=0,\boldsymbol{\theta},\cdot],
%	\end{align*}
	where $\mathbf{s}'_2 =(a_m+2,\mathbf{a}_{-m}',\mathbf{h}')$ and $\mathbf{s}'_1=(a_m+1,\mathbf{a}_{-m}',\mathbf{h}')$, and (b$'$) holds true because $V(a_m,\cdot)$ is non-decreasing in $a_m$ and due to \eqref{prob_rho}. 
	Now, to show that $I_{e,m}$ is non-decreasing in channel power gain $h_m$, it is sufficient to prove that $Q(\mathbf{a}, h_m, \mathbf{h}_{-m}, I_{e,m}, I_{l,m}=0, \mathbf{I}_{e,-m}, \mathbf{I}_{l,-m},\boldsymbol{\theta})$ is sub-modular in $(h_m,I_{e,m})$, when $\mathbf{a}, \mathbf{h}_{-m}, \mathbf{I}_{e,-m}, \mathbf{I}_{l,-m}$ are fixed. For some $\delta>0$, we have
	\begin{align}
		&Q(a_m, h_m+\delta, I_{e,m}=1, I_{l,m}=0,\boldsymbol{\theta},\cdot) \nonumber  \\
		& \qquad \qquad \qquad \qquad -  Q(a_m, h+\delta, I_{e,m}=0, I_{l,m}=0,\boldsymbol{\theta},\cdot) \nonumber  \\
		&= w_m +\lambda_mP_{e,m}(h_m+\delta) \nonumber \\
		&+\gamma\mathbb{E}\left[V(1,\mathbf{a}_{-m}',\mathbf{h}')|a_m, h_m+\delta, I_{e,m}=1, I_{l,m}=0,\boldsymbol{\theta},\cdot \right] \nonumber \\ 
		&- w_m ( a_m+1) \nonumber \\
		&- \gamma \mathbb{E}\left[V(\mathbf{s}')|a_m,  h_m+\delta, I_{e,m}=0, I_{l,m}=0, \boldsymbol{\theta} ,\cdot\right]\nonumber\\
		&\stackrel{c}{\leq} w_m +\lambda_mP_{e,m}(h_m) \nonumber \\ 
		&+\gamma\mathbb{E}\left[V(1,\mathbf{a}_{-m}',\mathbf{h}')|a_m, h_m, I_{e,m}=1, I_{l,m}=0,\boldsymbol{\theta},\cdot \right] \nonumber \\ 
		&- w_m (a_m+1) \nonumber \\
		&-\gamma \mathbb{E}\left[V(\mathbf{s}')|a_m, h_m, I_{e,m}=0, I_{l,m}=0,\boldsymbol{\theta},\cdot\right] \nonumber  \\
		%1+\gamma\mathbb{E}\left[V(1)\right] - \left( a+1 +\gamma \mathbb{E}\left[V(s')|a, I_e=0, I_l=0,\cdot\right]\right)\\
		&= Q(a_m, h_m, I_{e,m}=1, I_{l,m}=0,\boldsymbol{\theta},\cdot) \nonumber  \\
		& \qquad \qquad \qquad -  Q(a_m, h_m, I_{e,m}=0, I_{l,m}=0,\boldsymbol{\theta},\cdot),
	\end{align}
	where $\mathbf{s}' = (a_m+1,\mathbf{a}_{-m}',\mathbf{h}')$ and (c) holds true because, from \eqref{decoding_order},  $P_{e,m}(h_m+\delta) < P_{e,m}(h_m)$ and since the realizations of channel power gain are independent, for $x=h_m+\delta$ and $x=h_m$, $\mathbb{E}\left[V(a'_m,\mathbf{a}_{-m}',\mathbf{h}')|a_m, x, I_{e,m}, I_{l,m}=0,\boldsymbol{\theta},\cdot\right]$ is same, irrespective of whether $I_{e,m}=0$ or $I_{e,m}=1$. 
	
		\textit{Case 2:}  When $I_{l,m}=1$,
	to show   $I_{e,m}$ is non-decreasing in   $a_m$, it is sufficient to prove   $Q(a_m,\mathbf{a}_{-m}, \mathbf{h}, I_{e,m}, I_{l,m}=1, \mathbf{I}_{e,-m}, \mathbf{I}_{l,-m},\boldsymbol{\theta})$ is sub-modular in $(a_m,I_{e,m})$, when $\mathbf{a}_{-m}, \mathbf{h}, \mathbf{I}_{e,-m}, \mathbf{I}_{l,-m}$ are fixed. Consider %In the below, the fixed quantities are represented by $(.)$ for simplicity.
	\begin{align}
		&Q(a_m+1, I_{e,m}=1, I_{l,m}=1,\boldsymbol{\theta},\cdot) \nonumber  \\
		& \qquad \qquad \qquad \qquad  -  Q(a_m+1, I_{e,m}=0, I_{l,m}=1,\boldsymbol{\theta},\cdot) \nonumber  \\
		&= w_m +\lambda_m(P_{e,m}(h_m)+P_{l,m})  \nonumber  \\
		&+\gamma\mathbb{E}\left[V(1,\mathbf{a}_{-m}',\mathbf{h}')|a_m+1, I_{e,m}=1, I_{l,m}=1,\boldsymbol{\theta},\cdot \right] \nonumber \\ 
		&- (w_m + \lambda_mP_{l,m})  \nonumber  \\
		&-\gamma \mathbb{E}\left[V(1,\mathbf{a}_{-m}',\mathbf{h}')|a_m+1, I_{e,m}=0, I_{l,m}=1,\boldsymbol{\theta},\cdot\right]\nonumber\\
		&=  w_m +\lambda_m(P_{e,m}(h_m)+P_{l,m})  \nonumber  \\
		&+\gamma\mathbb{E}\left[V(1,\mathbf{a}_{-m}',\mathbf{h}')|a_m, I_{e,m}=1, I_{l,m}=1,\boldsymbol{\theta},\cdot \right] \nonumber \\ 
		&- ( w_m + \lambda_mP_{l,m})  \nonumber  \\
		&-\gamma \mathbb{E}\left[V(1,\mathbf{a}_{-m}',\mathbf{h}')|a_m, I_{e,m}=0, I_{l,m}=1,\boldsymbol{\theta},\cdot\right] \nonumber  \\
		%1+\gamma\mathbb{E}\left[V(1)\right] - \left( a+1 +\gamma \mathbb{E}\left[V(s')|a, I_e=0, I_l=0\right]\right)\\
		&= Q(a_m, I_{e,m}=1, I_{l,m}=1,\boldsymbol{\theta},\cdot) \nonumber  \\
		& \qquad \qquad \qquad \qquad -  Q(a_m, I_{e,m}=0, I_{l,m}=1,\boldsymbol{\theta},\cdot).
	\end{align}
	
	To show   $I_{e,m}$ is non-decreasing in   $h_m$, it is sufficient to prove   $Q(\mathbf{a}_m, h_m, \mathbf{h}_{-m}, I_{e,m}, I_{l,m}=1, \mathbf{I}_{e,-m}, \mathbf{I}_{l,-m},\boldsymbol{\theta})$ is sub-modular in $(h_m,I_{e,m})$, when $\mathbf{a}_m, \mathbf{h}_{-m}, \mathbf{I}_{e,-m}, \mathbf{I}_{l,-m}$ are fixed. For some $\delta>0$, we have
	\begin{align}
		&Q(a_m, h_m+\delta, I_{e,m}=1, I_{l,m}=1,\boldsymbol{\theta},\cdot) \nonumber  \\
		& \qquad \qquad \qquad  -  Q(a_m, h+\delta, I_{e,m}=0, I_{l,m}=1,\boldsymbol{\theta},\cdot) \nonumber  \\
		&= w_m +\lambda_m(P_{e,m}(h_m+\delta)+P_{l,m}) \nonumber  \\
		&+\gamma\mathbb{E}\left[V(1,\mathbf{a}_{-m}',\mathbf{h}')|a_m, h_m+\delta, I_{e,m}=1, I_{l,m}=1,\boldsymbol{\theta},\cdot \right] \nonumber \\ 
		&- (w_m  + \lambda_mP_{l,m}) \nonumber  \\
		&- \gamma \mathbb{E}\left[V(1,\mathbf{a}_{-m}',\mathbf{h}')|a_m,  h_m+\delta, I_{e,m}=0, I_{l,m}=1,\boldsymbol{\theta},\cdot\right]\nonumber\\
		&\stackrel{d}{\leq} w_m +\lambda_m(P_{e,m}(h_m)+P_{l,m}) \nonumber  \\
		&+\gamma\mathbb{E}\left[V(1,\mathbf{a}_{-m}',\mathbf{h}')|a_m, h_m, I_{e,m}=1, I_{l,m}=1,\boldsymbol{\theta},\cdot \right] \nonumber \\ 
		&-( w_m + \lambda_mP_{l,m}) \nonumber  \\
		&-\gamma \mathbb{E}\left[V(1,\mathbf{a}_{-m}',\mathbf{h}')|a_m, h_m, I_{e,m}=0, I_{l,m}=1,\boldsymbol{\theta},\cdot\right] \nonumber  \\
		%1+\gamma\mathbb{E}\left[V(1)\right] - \left( a+1 +\gamma \mathbb{E}\left[V(s')|a, I_e=0, I_l=0,\cdot\right]\right)\\
		&= Q(a_m, h_m, I_{e,m}=1, I_{l,m}=1,\boldsymbol{\theta},\cdot)  \nonumber  \\
		& \qquad \qquad \qquad -  Q(a_m, h_m, I_{e,m}=0, I_{l,m}=1,\boldsymbol{\theta},\cdot),
	\end{align}
	here (d) holds true because, from \eqref{decoding_order},  $P_{e,m}(h_m+\delta) < P_{e,m}(h_m)$ and since the realizations of channel power gain are independent, $\mathbb{E}\left[V(a'_m,\mathbf{a}_{-m}',\mathbf{h}')|a_m, x, I_{e,m}, I_{l,m}=1,\boldsymbol{\theta},\cdot\right]$ is same for $x=h_m+\delta$ and $x=h_m$, irrespective of whether $I_{e,m}=0$ or $I_{e,m}=1$.  Hence,  when $\mathbf{a}_{-m},
	\mathbf{h}$ and $\mathbf{I}_{e,-m}$, $\mathbf{I}_{l}$ are fixed, and for any arbitrary decoding order $\boldsymbol{\theta}$, the optimal action $I_{e,m}$ is non-decreasing in $a_m$. Similarly, when $\mathbf{a}, \mathbf{h}_{-m}$ and $\mathbf{I}_{e,-m}$, $\mathbf{I}_{l}$ are fixed, and for any arbitrary decoding order $\boldsymbol{\theta}$, the optimal action $I_{e,m}$ is non-decreasing in   $h_m$. 	
  Along the similar lines, we can prove that $I_{l,m}$ is non-decreasing in $a_m$ (and $h_m$) when other state-action variables are fixed. 
\end{proof}
\subsection{Proof of Theorem 3} \label{Thm:3}

	Prior to proving Theorem \ref{opt_ratio}, we obtain an upper bound to the conditional Lyapunov drift and show that the virtual queue, $Q_m(k),\; \forall m \in \{1,2,\dots,M\}$ is strongly stable. To compute an  upper bound on the conditional Lyapunov drift, we upper bound the change in the Lyapunov function as follows:
	\begin{align}
	& L(Q(k+1))  - L(Q(k)) = \frac{1}{2}\sum_{m=1}^{M} \left(Q^2_m(k+1) - Q^2_m(k)\right)\nonumber\\
	& = \frac{1}{2}\sum_{m=1}^{M} \left((\max\{Q_m(k)-\bar{P}_m, 0\} + P_m(k))^2 - Q^2_m(k)\right)\nonumber\\
	&\stackrel{b}\leq \frac{1}{2}\sum_{m=1}^{M}  \left( Q_m^2(k)+\bar{P}_m^2 + P_m^2(k) \right) \nonumber \\
	& +  \frac{1}{2}\sum_{m=1}^{M} \left( 2 Q_m(k) (P_m(k)- \bar{P}_m)- Q^2_m(k)\right)\nonumber\\
	\label{eq:UB-LF} & =  \sum_{m=1}^{M}  \left( \frac{\bar{P}_m^2 }{2}+ \frac{P_m^2(k)}{2} +  Q_m(k) \left(P_m(k)- \bar{P}_m\right)\right),
	%\right)+ \frac{1}{2}\sum_{m=1}^{M} \left(
	\end{align}
where (b) holds true   because $Q_m\geq 0, \bar{P}_m \geq 0, P_m\geq 0$ and  due to the following inequality, 
\begin{align}
	&(\max\{Q_m(k)-\bar{P}_m, 0\} + P_m(k))^2 \nonumber\\
	&\qquad \quad \leq  Q_m^2(k)+\bar{P}_m^2 + P_m^2(k) + 2 Q_m (k) (P_m(k)- \bar{P}_m).\nonumber
\end{align}
From \eqref{eq:UB-LF}, we have 
	\begin{align} 
	& \Delta(S(k)) \nonumber \\	
	&\leq \mathbb{E}\left[\sum_{m=1}^{M}  \left( \frac{\bar{P}_m^2 }{2}+ \frac{P_m^2(k)}{2} +  Q_m(k) \left(P_m(k)- \bar{P}_m\right)\right)\Big|S(k)\right] \nonumber \\
	&=\frac{1}{2}\sum_{m=1}^{M}\bar{P}_m^2 + \frac{1}{2}\sum_{m=1}^{M}\mathbb{E}\left[{P_m^2(k)}|S(k) \right] \nonumber \\ 
	& + \sum_{m=1}^{M}Q_m(k) \left(\mathbb{E}\left[P_m(k)|S(k)\right]- \bar{P}_m\right)\nonumber \\
	\label{upper_bound1}& \leq M B + \sum_{m=1}^{M} Q_m(k) (\mathbb{E}\left[P_m(k)|S(k)\right]- \bar{P}_m),
	\end{align}
where %$B \geq  \frac{1}{2 M}\sum_{m=1}^{M} \left(\bar{P}_m^2 +  \left(\max_{\boldsymbol{\theta},\mathbf{h}} \{P_{e,m}(h_m)\}_{m= 1}^{M}+P_{l,m}\right)^2\right)$.
\begin{align}
	B = \frac{1}{2 M}\sum_{m=1}^{M} \left(\bar{P}_m^2 +  \left(\max_{\boldsymbol{\theta},\mathbf{h}} \{P_{e,m}(h_m)\}_{m= 1}^{M}+P_{l,m}\right)^2\right) \nonumber. 
\end{align}

We now prove the strong stability of virtual queues:
\begin{lemma}
	The virtual queue $Q_m(k)$ is strongly stable, i.e.,
	\begin{align} \label{queue-stability}
		\lim_{K \to \infty}\frac{1}{K}\sum_{k=1}^{K}\mathbb{E}[Q_m(k)]<\infty, \;\; \forall m \in \{1,2,\dots, M\}.
	\end{align}
\end{lemma}
\begin{proof}
	To prove the strong stability of $Q_m(k)$, we assume that Slater's condition holds for \eqref{AoP}, i.e., there exists $\alpha > 0$, $\hat{A}(\alpha) \geq 0 $ and a channel-only policy such that in each slot,
 \begin{flalign}\label{slater}
    & \sum_{m=1}^{M}\mathbb{E}[w_m\hat{a}_m(k+1)] = \hat{A}(\alpha), \mathbb{E}[\hat{P}_m(k)] + \alpha \leq \bar{P}_m,&&
 \end{flalign}
	% \begin{align} \label{age_slater}
	% 	\sum_{m=1}^{M}\mathbb{E}[ w_m\hat{a}_m(k+1)] = \hat{A}(\alpha),
	% \end{align} 
% \begin{align}\label{power_slater}
	% 	\mathbb{E}\left[\hat{P}_m(k)\right] + \alpha \leq \bar{P}_m,
	% \end{align}
for all $m \in \{1,2,\dots, M\}$ and here $\hat{a}_m(k+1)$ denotes the AoPI of user $m$ in slot $k$ and $\hat{P}_m(k)$ denotes the power expended at user $m$ in slot $k$ for channel-only policy, the class of polices where the decision is made based on channel power gain vector, $\mathbf{h}(k)$ in slot $k$.
	From \eqref{upper_bound1}, we have, 
	$\Delta(S(k)) + \beta \sum_{m=1}^{M}\mathbb{E}[w_m a_m(k+1)|S(k)]
		 \stackrel{b} \leq MB + \sum_{m=1}^{M} Q_m(k) \left(\mathbb{E}\left[P_m(k)|S(k)\right]- \bar{P}_m\right)  + \beta \sum_{m=1}^{M}\mathbb{E}[w_m a_m(k+1)|S(k)] \stackrel{c}\leq M B + \sum_{m=1}^{M} Q_m(k)\left(\mathbb{E}\left[\hat{P}_m(k)|S(k)\right]- \bar{P}_m\right) + \beta \sum_{m=1}^{M}\mathbb{E}[w_m \hat{a}_m(k+1)|S(k)] \nonumber,
	$
	where (c) is due to \eqref{slater} and (c) holds true because, we minimize RHS of inequality (b) over all possible policies greedily and channel-only policy that results in \eqref{slater} is also a one among the possible policies. 
	Now, taking expectation over $S(k)$ and due to the law of iterated expectations, we have
	\begin{align}\label{eq:LB-channel-only}
		&\mathbb{E}[L(Q(k+1))] - \mathbb{E}[L(Q(k))] + \beta \sum_{m=1}^{M}\mathbb{E}[w_m a_m(k+1)] \nonumber\\
		&\stackrel{d}\leq M B - \alpha \sum_{m=1}^{M} \mathbb{E}[Q_m(k)] +  \beta \hat{A}(\alpha),
	\end{align}
	where (d) is true because, from \eqref{slater} for the channel-only policy $		\sum_{m=1}^{M}\mathbb{E}[w_m \hat{a}_m(k+1)|S(k)] = \hat{A}(\alpha)$ and 
	%\begin{align}\label{eq:power_slater_state_indp}
	$	\mathbb{E}\left[\hat{P}_m(k)|S(k)\right] + \alpha =\mathbb{E}\left[\hat{P}_m(k)\right] + \alpha \leq \bar{P}_m$. 	%\end{align}
 Substituting this in \eqref{eq:LB-channel-only} and summing over $\{1,\ldots, K\}$, we have
$\alpha \sum_{k=1}^K \sum_{m=1}^{M} \mathbb{E}[Q_m(k)]  \leq - \mathbb{E}[L(Q(K))] + \mathbb{E}[L(Q(1))] - \beta \sum_{k=1}^K\sum_{m=1}^{M}\mathbb{E}[w_m a_m(k+1)] + KB  +  \beta K \hat{A}(\alpha)   \stackrel{e} <  \mathbb{E}[L(Q(1))]  + K M B  +  \beta K \hat{A}(\alpha)$, 
	where (e) is obtained by discarding the negative terms,  $- \mathbb{E}[L(Q(K))]$, $- \beta \sum_{k=1}^K\sum_{m=1}^{M}\mathbb{E}[w_m a_m(k+1)]$ and since, $- \beta \sum_{k=1}^K\sum_{m=1}^{M}\mathbb{E}[w_m a_m(k+1)] < 0$. Further, dividing the entire equation by $K$, we have
	$\frac{\alpha}{K} \sum_{k=1}^K\sum_{m=1}^{M}\mathbb{E}[Q_m(k)] < M B +  \beta \hat{A}(\alpha) + \frac{\mathbb{E}[L(Q(1))]}{K}$.
%\begin{align} 
%		\frac{\alpha}{K} \sum_{k=1}^K\sum_{m=1}^{M}\mathbb{E}[Q_m(k)] < M B +  \beta \hat{A}(\alpha) + \frac{\mathbb{E}[L(Q(1))]}{K}. \nonumber
%	\end{align}
Now applying the limit $K \to \infty$ and   noting that 
$\mathbb{E}[L(Q(1))]$ is a finite value, we get
$\lim_{K \to \infty} \frac{1}{K} \sum_{k=1}^K\sum_{m=1}^{M}\mathbb{E}[Q_m(k)]  < \frac{ M B+ \beta \hat{A}(\alpha)}{\alpha}$.
% \begin{align}
% 		\lim_{K \to \infty} \frac{1}{K} \sum_{k=1}^K\sum_{m=1}^{M}\mathbb{E}[Q_m(k)]  < \frac{ M B+ \beta \hat{A}(\alpha)}{\alpha}. \nonumber
% \end{align}
  Since $B$ is a constant and $\alpha>0$, \eqref{queue-stability} follows.  %i.e., %$\hat{A}(\alpha)< \infty$,
 %the virtual queue $Q_m(k)$ is strongly stable.
\end{proof}
	We now show that there exists a channel-only policy to \eqref{AoP} that helps in obtaining an  upper bound to $A_{\rm DPP}$. %drift-plus-penalty method.   
	\begin{lemma}
		There exists a channel-only policy to \eqref{AoP} (when feasible) that satisfies: 
		\begin{align}
			\label{channel-only_age2}& \frac{1}{M} \sum_{m=1}^{M}\mathbb{E}[w_m \tilde{a}_{{m}}(k)]\leq  A^* + \delta,\\
			\label{channel-only_power2}&\mathbb{E}[\tilde{P}_m(k)]-\bar{P}_m \leq \delta,\;\; \forall  m = 1,2,\ldots,M,
		\end{align}
		for any $\delta\geq 0$, where $\tilde{a}_{{m}}(k)$ is the AoPI and $\tilde{P}_m(k)$ is the power consumed by user $m$ under the channel-only policy, and $A^*$ is the optimal objective value of \eqref{AoP}. 
	\end{lemma}
	\begin{proof}
	Note that $\mathbb{E}[P_m^2(k)] \leq \left({\max_{\boldsymbol{\theta}, \mathbf{h}}} \{P_{e,m}(h)\}_{m= 1}^{M}+P_{l,m}\right)^2$ and the channel gains, $h_m(k)$ are i.i.d. over slots.  Further,    \eqref{eq:DPP_greedy} is feasible if $1\leq a_m(k) < \infty$.  Therefore, the result follows for $\delta>0$ from Theorem 4.5 in \cite{Neely}, as the above conditions satisfies the conditions for which the theorem is stated.   Moreover, the one-slot expectations $\mathbb{E}[w_m \tilde{a}_{{m}}(k)]$ and $\mathbb{E}[\tilde{P}_m(k)]$ are finite, as the event space, $\mathcal{H}$ and the action space, $\{(a,b,c)\}^M$, where $a,b\in \{0,1\}$ and $c \in \{1,2,\dots,M\}$ are finite (and hence closed). Hence, the result follows for $\delta=0$ case.  
	\end{proof}
Now, we prove Theorem \ref{opt_ratio} as follows:
\begin{proof}
 We first obtain an upper bound to the optimal objective function of the drift-plus-penalty problem \eqref{DPP}, which helps in bounding the long-term weighted average AoPI of the DPP policy, $A_{\rm DPP}$. From the upper bound in \eqref{upper_bound1}, we have
	%For the optimal solution to \eqref{DPP}, we have the following: 
	$\Delta(S(k)) + \beta \sum_{m=1}^{M}\mathbb{E}[w_m a_m(k+1)|S(k)]  \leq M B + \sum_{m=1}^{M} Q_m(k) \left(\mathbb{E}\left[P_m(k)|S(k)\right]- \bar{P}_m\right) + \beta \sum_{m=1}^{M}\mathbb{E}\left[w_m a_m(k+1)|S(k)\right]   
	 \stackrel{b}\leq MB + \sum_{m=1}^{M} Q_m(k) \left(\mathbb{E}\left[\tilde{P}_m(k)\right]- \bar{P}_m\right) + \beta \sum_{m=1}^{M}\mathbb{E}\left[w_m\tilde{a}_m(k+1)\right]  \stackrel{c} \leq M B + \sum_{m=1}^{M} Q_{m}(k) \delta + \beta ( M A^*+  M\delta),$
%	\begin{align}\label{eq:Bound}
%	&	\Delta(S(k)) + \beta \sum_{m=1}^{M}\mathbb{E}[w_m a_m(k+1)|S(k)]\nonumber\\
%		& \leq M B + \sum_{m=1}^{M} Q_m(k) \left(\mathbb{E}\left[P_m(k)|S(k)\right]- \bar{P}_m\right) \nonumber \\ 
%		& + \beta \sum_{m=1}^{M}\mathbb{E}\left[w_m a_m(k+1)|S(k)\right]\nonumber\\
%		& \stackrel{b}\leq MB + \sum_{m=1}^{M} Q_m(k) \left(\mathbb{E}\left[\tilde{P}_m(k)\right]- \bar{P}_m\right) \nonumber \\
%		& + \beta \sum_{m=1}^{M}\mathbb{E}\left[w_m\tilde{a}_m(k+1)\right]\nonumber\\
%		&  \stackrel{c} \leq M B + \sum_{m=1}^{M} Q_{m}(k) \delta + \beta ( M A^*+  M\delta),
%	\end{align}
  where (b) is because, we minimize RHS of the upper bound to $\Delta(S_k)$ over all possible policies greedily and channel-only policy which is independent of state $S(k)$ and satisfies \eqref{channel-only_age2} and \eqref{channel-only_power2}, is a permissible policy. %and hence \eqref{eq:age_slater_state_indp} and \eqref{eq:power_slater_state_indp} can be used. 
Here, (c) holds true due to \eqref{channel-only_age2}.
As $\delta\rightarrow 0$, %({\color{blue}$\delta=0$ holds when actions are finite}), 
we have $\Delta(S(k)) + \beta \sum_{m=1}^{M}\mathbb{E}\left[w_m a_m(k+1)|S(k)\right] \leq M B + \beta M A^*$.
Taking expectation over $S(k)$, we have
\begin{align}\label{eq:LB-channel-only2}
	&\mathbb{E}[L(Q(k+1))] - \mathbb{E}[L(Q(k))] + \beta \sum_{m=1}^{M}\mathbb{E}[ w_m a_m(k+1)] \nonumber \\ &\leq  M B + \beta M A^*. 
\end{align}
Summing the above expression over $\{1,2,\dots,K\}$ and rearranging the terms, we have $\beta \sum_{k=1}^{K}\sum_{m=1}^{M}\mathbb{E}[ w_m a_m(k+1)] \leq -\mathbb{E}[L(Q(K))] + \mathbb{E}[L(Q(1))] + K M B + \beta K M A^* \stackrel{d}\leq \mathbb{E}[L(Q(1))] + K M B + \beta K  M A^*,$
%\begin{align}
%	&\beta \sum_{k=1}^{K}\sum_{m=1}^{M}\mathbb{E}[ w_m a_m(k+1)] \nonumber \\ 
%	& \leq -\mathbb{E}[L(Q(K))] + \mathbb{E}[L(Q(1))] + K M B + \beta K M A^* \nonumber \\
%	& \stackrel{d}\leq \mathbb{E}[L(Q(1))] + K M B + \beta K  M A^*,
%\end{align}
where (d) is obtained by discarding the negative term,  $- \mathbb{E}[L(Q(K))]$. Dividing the entire equation by $MK$,  applying limit $K \to \infty$ and  noting that  $\mathbb{E}[L(Q(1))]$ is finite, we get
\begin{align}\label{age_opt_dpp1}
		A_{\rm DPP} = \lim_{K \to \infty} \frac{1}{MK} \sum_{k=1}^K\sum_{m=1}^{M}\mathbb{E}[w_m a_m(k+1)] \leq \frac{B}{\beta} + A^*. 
	\end{align} 
We now obtain a lower bound, $A_L$ to $A^*$ of \eqref{AoP} that helps in proving the theorem. Let ${\mathbf{I}^{L}_{e}(k),\mathbf{I}^{L}_{l}(k)},\boldsymbol{\theta}^{L}(k)$ be the optimal action for slot $k$ obtained by solving \eqref{AoP_LB}. Let $u^L_m(k)$ be equal to $1$, if user $m$ receives a processed packet successfully in slot $k$ either from the local processor or the edge processor, else $u^L_m(k)$ is equal to $0$, under the optimal actions.  The corresponding optimal objective value, $A_L$ is given by
\begin{align}
	\label{eq:Age-LB-Appendix} A_L = & \lim_{K \to \infty}\frac{1}{2M}\sum_{m=1}^{M} w_m \left(\frac{1}{\frac{1}{K}\sum_{k=1}^{K} \mathbb{E}\left[u_m^{L}(k)\right]}+1\right),
\end{align}
where $k \in \{1,2,\dots\}$ and $m=\{1,2,\dots,M\}$. 
 Since, the constraints for lower bound optimization problem, \eqref{AoP_LB} and that for the original optimization problem, \eqref{AoP} are identical, the optimal policy of \eqref{AoP_LB} is a feasible policy for \eqref{AoP}. Using the optimal policy of \eqref{AoP_LB} and evaluating \eqref{AoP} we get 
	\begin{equation}\label{LB_age}
		A = \lim_{K \to \infty}\frac{1}{M}\sum_{m=1}^{M} w_m \left(\frac{1}{\frac{1}{K}\sum_{k=1}^{K} \mathbb{E}\left[u_m^{L}(k)\right]}\right).
	\end{equation}
As the optimal policy for 	\eqref{AoP_LB} may not be optimal for \eqref{AoP}, we have, $A\geq A^*$. From \eqref{age_opt_dpp1}: 
	\begin{equation}\label{DPP_age}
		A_{\rm DPP} \leq \frac{B}{\beta} + A^* \leq \frac{B}{\beta} + A.
	\end{equation}
	Using \eqref{eq:Age-LB-Appendix}, \eqref{LB_age} and \eqref{DPP_age}, we get $A_L \leq A_{\rm DPP} \leq \frac{B}{\beta} + 2A_L - 1$. Therefore, the optimality ratio is
	\begin{equation}
		%\rho_{\rm DPP} = 
		\frac{A_{\rm DPP}}{A^*} \leq \frac{A_{\rm DPP}}{A_L} \leq 2 + \frac{1}{A_L}\left(\frac{B}{\beta} - 1\right).
	\end{equation}
\end{proof}
